# Supplementary material for: Structural defects responsible for strain glassy transition in Ni$_{50+x}$Ti$_{50-x}$
Source: arXiv:2103.07103 source file (2021-03-12)
Supplement: Supplementary file 1 [file Supplementary.pdf]

*Supplementary material to the paper titled*

**Structural defects responsible for strain glassy transition in $Ni_{50+x}Ti_{50-x}$**

TABLE I. The results of the best fits obtained at 300K and 77K for the four alloy compositions at Ti edge carried out in the $k$-range 3-12 $Å^{-1}$, $k$ weighted at 2 and in $R$-range 1-3 Å. The bond length is given by the parameter $R$ while the thermal variation in bond length is described by $\sigma^2$. Figures in parenthesis indicate uncertainty in last digit.

| **Alloys** | **Atoms with coordination no.** | **300K** R(Å) | **300K** $\sigma^2$ (Å$^2$) | **77K** R(Å) | **77K** $\sigma^2$ (Å$^2$) |
|---|---|---|---|---|---|
| NT50 | Ni1×3 | 2.49(1) | 0.0175(8) | 2.49(1) | 0.016(1) |
| | Ni2×4 | 2.58(1) | 0.0175(8) | 2.58(1) | 0.016(1) |
| | Ti1×2 | 2.86(2) | 0.004(1) | 2.86(2) | 0.002(2) |
| | Ti2×2 | 3.00(2) | 0.005(2) | 3.00(3) | 0.004(2) |
| NT52 | Ni1×3 | 2.49(3) | 0.017(2) | 2.49(2) | 0.015(1) |
| | Ni2×4 | 2.58(3) | 0.017(2) | 2.58(2) | 0.015(1) |
| | Ti1×2 | 2.88(4) | 0.005(4) | 2.87(2) | 0.004(3) |
| | Ti2×2 | 3.03(6) | 0.008(5) | 3.02(4) | 0.007(4) |
| NT55 | Ni1×3 | 2.49(3) | 0.013(2) | 2.49(3) | 0.011(2) |
| | Ni2×4 | 2.58(3) | 0.013(2) | 2.58(3) | 0.011(2) |
| | Ti1×2 | 2.88(3) | 0.004(3) | 2.88(3) | 0.003(3) |
| | Ti2×2 | 3.04(6) | 0.007(5) | 3.04(3) | 0.005(5) |
| NT60 | Ni1×3 | 2.496(6) | 0.0104(8) | 2.51(2) | 0.008(1) |
| | Ni2×4 | 2.584(6) | 0.0104(8) | 2.59(2) | 0.008(1) |
| | Ti1×2 | 2.89(1) | 0.004(2) | 2.90(1) | 0.003(2) |
| | Ti2×2 | 3.07(3) | 0.009(5) | 3.09(3) | 0.010(4) |

TABLE II. The results of the best fits obtained at 300K and 77K for the four alloy compositions at Ni edge carried out in the $k$-range 3-12 Å$^{-1}$, $k$ weighted at 2 and in $R$-range 1-3.5 Å. The bond length is given by the parameter $R$ while the thermal variation in bond length is described by $\sigma^2$. Figures in parenthesis indicate uncertainty in last digit.

| **Alloys** | **Atoms with coordination no.** | **300K** R(Å) | $\sigma^2$ (Å$^2$) | **77K** R(Å) | $\sigma^2$ (Å$^2$) |
|---|---|---|---|---|---|
| NT50 | Ti1×3 | 2.51(3) | 0.032(2) | 2.51(3) | 0.032(2) |
| | Ti2×4 | 2.60(3) | 0.032(2) | 2.60(3) | 0.032(2) |
| | Ni1×2 | 2.63(3) | 0.017(3) | 2.61(3) | 0.017(3) |
| | Ni2×2 | 2.90(3) | 0.017(3) | 2.88(3) | 0.017(3) |
| | Ni1×8 (Ni BCC) | 2.45(1) | 0.007(2) | 2.45(1) | 0.007(2) |
| NT52 | Ti1×3 | 2.51(5) | 0.031(2) | 2.51(4) | 0.031(2) |
| | Ti2×4 | 2.60(5) | 0.031(2) | 2.60(4) | 0.031(2) |
| | Ni1×2 | 2.63(5) | 0.018(6) | 2.61(4) | 0.018(5) |
| | Ni2×2 | 2.90(5) | 0.018(6) | 2.88(4) | 0.018(5) |
| | Ni1×8 (Ni BCC) | 2.461(8) | 0.008(2) | 2.464(6) | 0.007(7) |
| NT55 | Ti1×3 | 2.52(6) | 0.032(3) | 2.52(6) | 0.031(3) |
| | Ti2×4 | 2.61(6) | 0.032(3) | 2.60(6) | 0.031(3) |
| | Ni1×2 | 2.63(7) | 0.019(8) | 2.62(6) | 0.019(8) |
| | Ni2×2 | 2.90(7) | 0.019(8) | 2.89(6) | 0.019(8) |
| | Ni1×8 (Ni BCC) | 2.481(8) | 0.008(2) | 2.482(7) | 0.0073(8) |
| NT60 | Ti1×8 | 2.64(2) | 0.046(2) | 2.63(8) | 0.036(4) |
| | Ni1×6 | 3.11(5) | 0.048(9) | 3.01(8) | 0.030(9) |
| | Ni1×12 (Ni FCC) | 2.513(2) | 0.0083(5) | 2.514(3) | 0.0063(4) |
| | Ni2×6 (Ni FCC) | 3.54(2) | 0.015(3) | 3.57(3) | 0.012(4) |

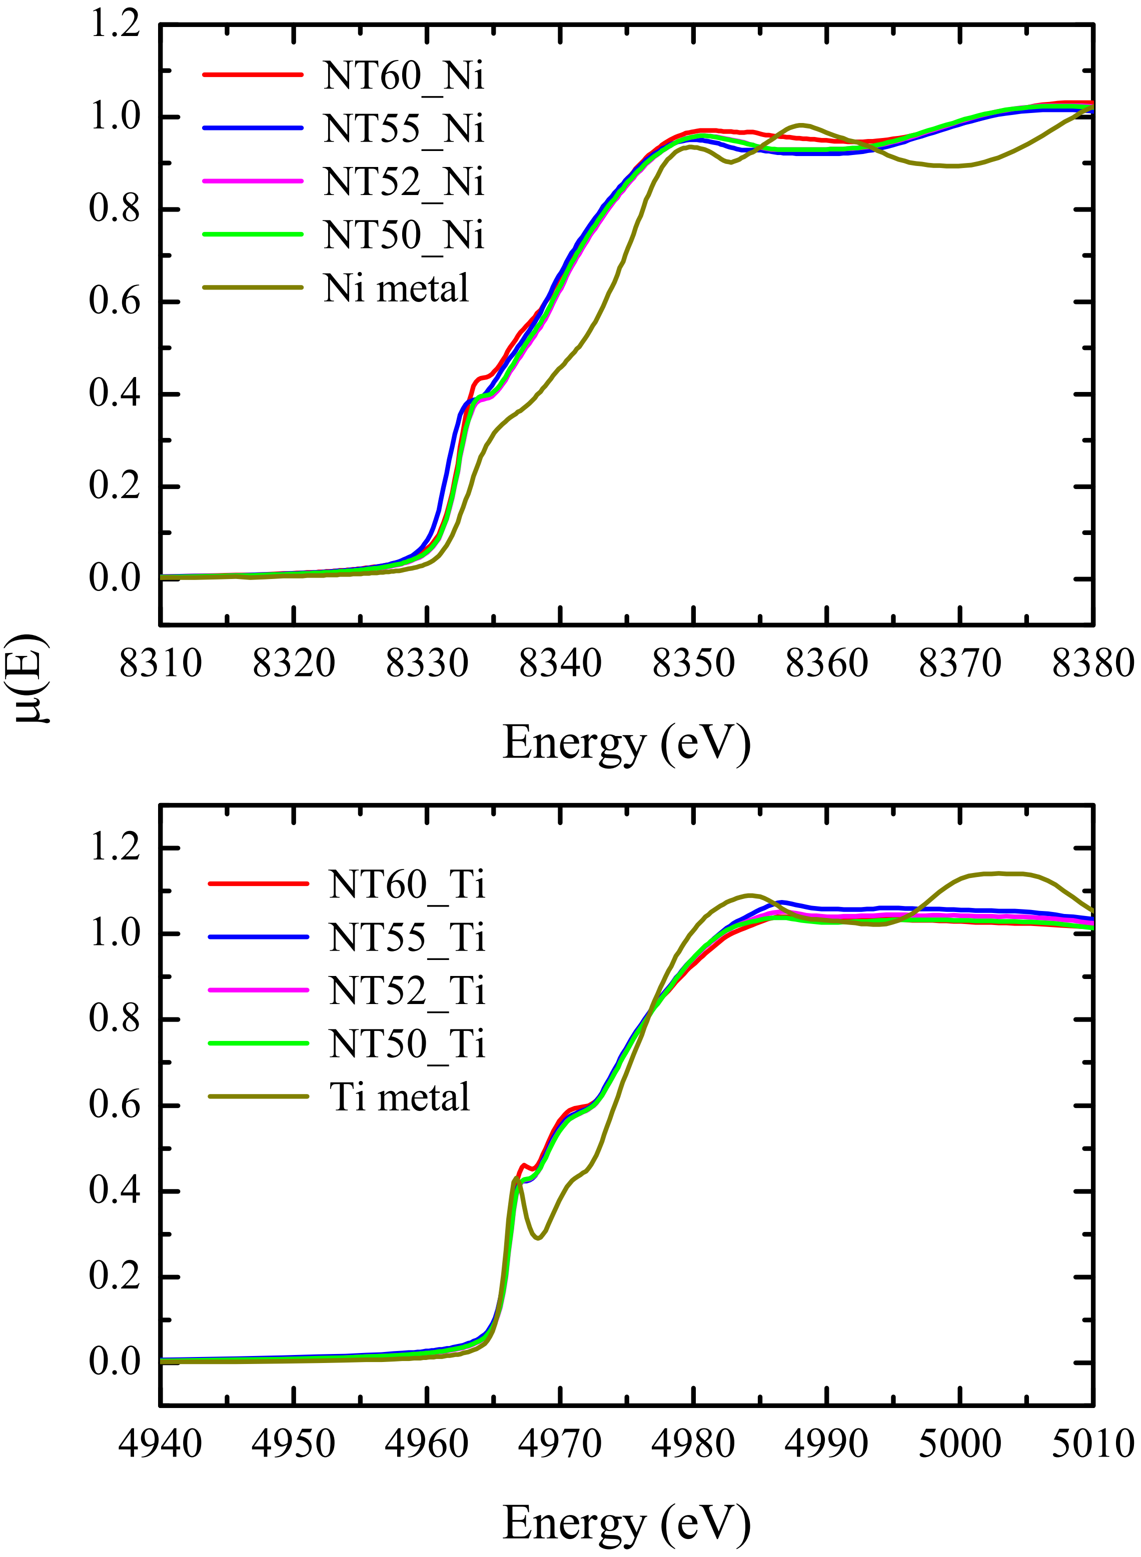


FIG. 1. The near edge data for Ni and Ti metal compared with the respective near edge data in the four alloy compositions.
